# Supplementary material for: Low-Rank Sinkhorn Factorization
Source: arXiv:2103.04737 source file (2021-03-08)
Supplement: Supplementary file 1 [file supplement.tex]

% \documentclass[twoside]{article}

% \usepackage{aistats2021}
% If your paper is accepted, change the options for the package
% aistats2021 as follows:
%
%\usepackage[accepted]{aistats2021}
%
% This option will print headings for the title of your paper and
% headings for the authors names, plus a copyright note at the end of
% the first column of the first page.

% If you set papersize explicitly, activate the following three lines:
%\special{papersize = 8.5in, 11in}
%\setlength{\pdfpageheight}{11in}
%\setlength{\pdfpagewidth}{8.5in}

% If you use natbib package, activate the following three lines:
%\usepackage[round]{natbib}
%\renewcommand{\bibname}{References}
%\renewcommand{\bibsection}{\subsubsection*{\bibname}}

% If you use BibTeX in apalike style, activate the following line:
%\bibliographystyle{apalike}

% \begin{document}

% If your paper is accepted and the title of your paper is very long,
% the style will print as headings an error message. Use the following
% command to supply a shorter title of your paper so that it can be
% used as headings.
%
%\runningtitle{I use this title instead because the last one was very long}

% If your paper is accepted and the number of authors is large, the
% style will print as headings an error message. Use the following
% command to supply a shorter version of the authors names so that
% they can be used as headings (for example, use only the surnames)
%
%\runningauthor{Surname 1, Surname 2, Surname 3, ...., Surname n}

% Supplementary material: To improve readability, you must use a single-column format for the supplementary material.
\onecolumn
\onecolumn
\section*{Supplementary material}

\section{Notations}
Let $I\geq 1$ and let us denote $(P^{(\ell)})_{0\leq \ell\leq I}$ the sequence of coupling obtained from Algorithm~(\ref{alg-mirror-descent}) with initialization $P^{(0)}:=a b^T$. Denote also $K^{(\ell)}:=\exp(- C^{(\ell)}/\varepsilon)$ where $C^{(\ell)}:= - 4 D P^{(\ell)} D'$. Moreover in the following we define for any $P,Q\in\mathbb{R}^{n\times m}$
\begin{align*}
    C(P):= - 4 D P D'  \text{\quad and \quad}  K(Q):=\exp(-Q/\varepsilon).
\end{align*}
Moreover for any $C\in\mathbb{R}^{n\times m}$, we denote:
\begin{align*}
    f_{C}(P):= \langle P,C \rangle - \varepsilon H(P)
\end{align*}
and 
\begin{align*}
    \Pi(C):= \argmin_{P\in\Pi(a,b)} f_{C}(P).
\end{align*}

\section{Quadratic Time Gromov-Wasserstein Distance}
\label{sec:quad-GW}
\begin{thm}
\label{thm:quadratic-GW}
Let $I\geq 1$ and $0<\delta\leq 1$. If for all $\ell\in\{0,..,I-1\}$
\begin{align*}
   \mu_\ell&:=\frac{\varepsilon \delta_\ell^2}{24\left[R + 1 +  \log\left(\frac{2\max(n,m)}{\delta_\ell^2}\right)\right] + 200}\\
   \delta_\ell&:=\min\left(\frac{\delta}{2L I},\frac{\delta}{2L I(R/\varepsilon)^{I-(\ell+1)}}]\right)\\
   L&:=\sup_{i,j,k,l}|D_{i,k}-D_{j,j}|^2 \text{\quad and \quad}  R:=4 \Vert D\Vert_{\text{op}}\Vert D'\Vert_{\text{op}}
\end{align*}
then the Gromov-Wasserstein Algorthm.~(\ref{alg-quad-GW}) with input $P^{(0)}$ outputs an approximation of the GW distance $\widehat{\mathcal{E}}$ and the coupling $\widehat{P}$ such that:
\begin{align*}
    \Vert P^{(I)} - \widehat{P}\Vert_1&\leq \frac{\delta}{2L}\\
    |\mathcal{E}_{D,D'}(P^{(I)}) - \widehat{\mathcal{E}}|&\leq \delta
\end{align*}
in $\mathcal{O}(n^2 (Ir + T)+ nr^2 + r^3 )$ algebraic operations where $T\in\mathcal{O}\left(I\mu_0^{-1}\left[\varepsilon^{-1} R +\log(\iota^{-1})\right]\right)$  and $(P^{(\ell)})_{0 \leq \ell\leq I}$ is the sequence obtained from Algorithm~(\ref{alg-mirror-descent}).
\end{thm}

\begin{proof}
Let us first introduce some notations to denote the sequences of coupling $Q^{(\ell)}$ obtained from Algorithm~(\ref{alg-quad-GW}). Indeed let $I\geq 1$, $(\mu_{\ell})_{1\leq \ell \leq I-1}\in (0,1)^I$ and let us now define the following sequence of matrices. Denote $Q^{(0)}:=P^{(0)}$, $C_1^{(0)}:=C^{(0)}$ , $K_1^{(0)} = K^{(0)}$ and define for $\ell=0,..,I-1$:
\begin{align*}
\label{def-approx-quad-GW}
    u^{(\ell+1)},v^{(\ell+1)}&:=\text{Sinkhorn}(K_1^{(\ell)},a,b,\mu_\ell)\\
    Q^{(\ell+1)}&:= \text{Diag}(u^{(\ell+1)})  K_1^{(\ell)}  \text{Diag}(v^{(\ell+1)})\\
    C_1^{(\ell+1)} &= - 4 D Q^{(\ell+1)} D'\\
    K_1^{(\ell+1)}&:= \exp(-C_1^{(\ell+1)}/\varepsilon)
\end{align*}

\begin{lemma}
\label{lem:total-error-quad}
Let $I\geq 1$, $(\mu_k)_{0\leq k \leq I-1}\in (0,1)^I$ and let us denote $(Q^{(k)})_{0\leq k \leq I}$ the sequence of coupling obtained from Algorithm~(\ref{alg-quad-GW}). Then for any $k\in\{1,...,I\}$, we have:
\begin{align*}
    \Vert P^{(k)} - Q^{(k)}\Vert_1\leq \sum_{j=1}^k \alpha^{j-1} \beta_{k-j}
\end{align*}
where for all $j=0,...,I-1$
\begin{align*}
    \alpha&:= \frac{4 \Vert D\Vert_{\text{op}}\Vert D'\Vert_{\text{op}}}{\varepsilon}\\
    \beta_j&:= \mu_j +\sqrt{\frac{4}{\varepsilon}\left[\mu_j \Vert C_1^{(k)}\Vert_{\infty}+ \varepsilon\mu_j\log\left(\frac{2\max(n,m)}{\mu_j}\right)\right]}
\end{align*}
\end{lemma}

\begin{prv}
First remarks that  $\delta_0:=\Vert P^{(0)} - Q^{(0)}\Vert_1=0$.
Let $k\in\{1,...,I-1\}$ and let us denote $\delta_k:=\Vert P^{(k)} - Q^{(k)}\Vert_1$. We have that
\begin{align*}
    \Vert P^{(k+1)} - Q^{(k+1)}\Vert_1\leq  \Vert P^{(k+1)} - \Pi(C(Q^{(k)})))\Vert_1 +
    \Vert \Pi(C(Q^{(k)})) - Q^{(k+1)} \Vert_1 
\end{align*}
Recall that $P^{(k+1)}=\Pi(C(P^{(k)})))$, therefore from Lemma~\ref{lem:error-cost}, we have first that:
\begin{align*}
     \Vert P^{(k+1)} - \Pi(C(Q^{(k)})))\Vert_1 \leq \frac{4\delta_k}{\varepsilon}\Vert D\Vert_{\text{op}}\Vert D'\Vert_{\text{op}}
\end{align*}
Moreover thanks Theorem 1 \todo{add prop in the main text at the end} in~\cite{dvurechensky2018computational}, we obtain that the Sinkhorn algorithm~\ref{alg-sink} outputs $u^{(k+1)},v^{(k+1)}$ such that $ Q^{(k+1)}:=\text{Diag}(u^{(k+1)}) K_1^{(k)}\text{Diag}(v^{(k+1)})$ satisfies $\Vert Q^{(k+1)}\mathbf{1}_n-a\Vert_1+ \Vert (Q^{(k+1)})^{T}\mathbf{1}_m-b\Vert_1\leq \mu_k$ in $\mathcal{O}\left(\mu_k^{-1}\log\left(\frac{1}{\iota \min_{i,j} K_1^{(k)}[i,j]}\right)\right)$ iterations where $\iota =\min\limits_{i,j}(a_i,b_j)$. Therefore thanks to Lemma~\ref{lem:error-sinkhorn}, we have finally that 
\begin{align*}
     \Vert \Pi(C(Q^{(k)})) -  Q^{(k+1)} \Vert_1\leq  \mu_k + \sqrt{\frac{4}{\varepsilon}\left[ \mu_k (\Vert C_1^{(k)} \Vert_{\infty} + \varepsilon \mu_k \log\left(\frac{2\max(n,m)}{ \mu_k }\right) \right]}
\end{align*}
Therefore we obtain that
\begin{align*}
    \delta_{k+1}:=  \Vert P^{(k+1)} - Q^{(k+1)}\Vert_1\leq \alpha \delta_k + \beta_k
\end{align*}
from which the result follows by a simple induction.
\end{prv}

\begin{prop}
\label{prop:l1-error-quad}
Let $I\geq 1$ and $0<\delta\leq 1$. If for all $k\in\{0,..,I-1\}$
$$\mu_k:=\frac{\varepsilon \delta_k^2}{200\left[R + 1 +  \log\left(\frac{2\max(n,m)}{\delta_k^2}\right)\right]}$$ where $$\delta_k:=\min\left(\frac{\delta}{I},\frac{\delta}{I\alpha^{I-(k+1)}}\right)$$, then we have that:
\begin{align*}
    \Vert P^{(I)} - Q^{(I)}\Vert_1\leq \delta
\end{align*}
\end{prop}

\begin{prv}
First remarks that for all $k\in\{0,,...,I-1\}$,
\begin{align*}
    \Vert C_1^{(k)}\Vert_{\infty}\leq \Vert C_1^{(k)}\Vert_{\text{op}} \leq R:=4 \Vert D\Vert_{\text{op}}\Vert D'\Vert_{\text{op}}
\end{align*}
and we obtain that 
\begin{align*}
     \beta_{k}\leq  \mu_k +\sqrt{\frac{4}{\varepsilon} \mu_k R}+ \sqrt{4\mu_k\log\left(\frac{2\max(n,m)}{\mu_k}\right)}
\end{align*}
Moreover as $\mu_k\leq 1$, we have that 
\begin{align*}
     \beta_{k}\leq  \mu_k +\sqrt{\frac{4}{\varepsilon} \mu_k R }+ \sqrt{4\mu_k\log\left(\frac{8\max(n,m)}{\delta_k^2}\right)} + \sqrt{4\frac{\mu_k}{\delta_k^2}\log\left(\frac{\delta_k^2}{4\mu_k}\right)}\delta_k
\end{align*}
Finally by considering 
\begin{align*}
    \mu_k\leq \min\left(\frac{\delta_k}{6},\frac{\varepsilon \delta_k^2}{144 R}, \frac{\delta_k^2}{144\log\left(\frac{2\max(n,m)}{\delta_k^2}\right)}, \frac{\delta_k^{2}}{200}\right) 
\end{align*}
we obtain that, 
\begin{align*}
     \mu_k &\leq \frac{\delta_k}{6}\\
     \sqrt{\frac{4}{\varepsilon} \mu_k R}&\leq  \frac{\delta_k}{6}\\
     \sqrt{4\mu_k\log\left(\frac{2\max(n,m)}{\delta_k^2}\right)} &\leq \frac{\delta_k}{6}
\end{align*}
Moreover as soon as $$\mu_k\leq \frac{\delta_k^{2}}{200}$$, we have that 
\begin{align*}
    4\frac{\mu_k}{\delta_k^2}\leq \frac{1}{50}&\implies 4\frac{\mu_k}{\delta_k^2}\log\left(\frac{\delta_k^2}{4\mu_k}\right)\leq \frac{1}{10}\\
    &\implies 
    \sqrt{4\frac{\mu_k}{\delta_k^2}\log\left(\frac{\delta_k^2}{\mu_k}\right)}\delta_k \leq \frac{\delta_k}{\sqrt{10}}\leq \frac{2\delta_k}{6}   
\end{align*}
Therefore we obtain that for such $\mu_k$, $\beta_k\leq \delta_k$. Finally by an union bound and by applying Lemma~\ref{lem:total-error}, we obtain that 
\begin{align*}
        \Vert P^{(I)} - Q^{(I)}\Vert_1\leq \delta
\end{align*}
\end{prv}
We can now prove the theorem. Let $\delta>0$. Thanks to Proposition~\ref{prop:l1-error-quad}, by considering for all $k\in\{0,..,I-1\}$
$$\mu_k:=\frac{\varepsilon \delta_k^2}{200\left[R + 1 +  \log\left(\frac{2\max(n,m)}{\delta_k^2}\right)\right]}$$ where $$\delta_k:=\min\left(\frac{\delta}{2LI},\frac{\delta}{2LI\alpha^{I-(k+1)}}\right)$$, then we have that:
we have that:
\begin{align*}
    \Vert P^{(I)} - Q^{(I)}\Vert_1\leq \frac{\delta}{2L}
\end{align*}
Finally applying Lemma~\ref{lem:GW-error} we obtain that 
\begin{align*}
     |\mathcal{E}_{D,D'}(P^{(I)}) - \mathcal{E}_{D,D'}(Q^{(I)})|&\leq \delta
\end{align*}

\begin{rmq}
At each iteration $k\in\{0,..,I-1\}$, the total number of iterations of the Sinkhorn algorithm is given by
$$T_k \in\mathcal{O}\left(\mu_k^{-1}\log\left(\frac{1}{\iota \min_{i,j} [K_1^{(k)}]_{ij}}\right)\right)$$.
First remarks that
$$\log\left(\frac{1}{\min_{i,j} [K_1^{(k)}]_{ij}}\right)\leq \varepsilon^{-1} \Vert C_1^{(k)}\Vert_\infty^2 \leq \varepsilon^{-1} R $$
Moreover note that as $k$ increases, $\mu_k$ decreases, therefore we have that for all $k\in\{0,..,I-1\}$, 
$$T_k \in \tilde{\mathcal{O}}\left(\left(\frac{LIR^I}{\varepsilon^I\delta}\right)^2\right)$$
where the notation $\tilde{\mathcal{O}}(.)$ means that we omits polylogarithmic factors w.r.t the constants of the problem.
\end{rmq}

\end{proof}

\section{Proof of Theorem~\ref{thm:rf-approx}}

\begin{proof}
Let us introduce some notations to denote the sequences of coupling $Q^{(k)}$ obtained from Algorithm~(\ref{alg-lin-GW}). Indeed let $I\geq 1$, $(r_k)_{0\leq k \leq I-1}\in\mathbb{N}^{I}$ $(\mu_{k})_{1\leq \ell \leq I-1}\in (0,1)^I$ and let us now define the following sequence of matrices. Denote $Q^{(0)}:=P^{(0)}$, $U^{(0)}:=A^{T}ab^TBB^{T}$,  $K_1^{(0)}=K^{(0)}$ and define for $k=0,..,I-1$:
\begin{align*}
    V_1^{(k)}, V_2^{(k)}&:=\text{RF-Approx}(4A,U^{(k)},r_k)\\
    \widehat{K_1}^{(k)}&:= V_1^{(k)} V_2^{(k)}\\
   u^{(k+1)},v^{(k+1)}&:=\text{Sinkhorn}(V_1^{(k)},V_2^{(k)},a,b,\mu_k)\\
   Q^{(k+1)} & = \text{Diag}(u^{(k+1)}) V_1^{(k)} V_2^{(k)} \text{Diag}(v^{(k+1)})\\
    K_1^{(k+1)}&:= \exp(- 4 D Q^{(k+1)} D'/\varepsilon)\\
    U^{(k+1)}&:= A^{T}  Q^{(k+1)} BB^{T} 
\end{align*}

\begin{lemma}
\label{lem:total-error}
Let $I\geq 1$, $(r_k)_{0\leq k \leq I-1}\in\mathbb{N}^{I}$ , and $(\mu_k)_{0\leq k \leq I-1}\in (0,1)^I$ and let us denote $(Q^{(k)})_{0\leq k \leq I}$ the sequence of coupling obtained from Algorithm~(\ref{alg-lin-GW}). Then for any $k\in\{1,...,I\}$, we have:
\begin{align*}
    \Vert P^{(k)} - Q^{(k)}\Vert_1\leq \sum_{j=1}^k \alpha^{j-1} \beta_{k-j}
\end{align*}
where for all $j=0,...,I-1$
\begin{align*}
    \alpha&:= \frac{4 \Vert D\Vert_{\text{op}}\Vert D'\Vert_{\text{op}}}{\varepsilon}\\
    \beta_j&:=\Vert \log(K_1^{(j)}/\widehat{K_1}^{(j)})\Vert_{\infty} + \mu_j +\sqrt{\frac{4}{\varepsilon}\left[\mu_j \Vert \widehat{C_1}^{(k)}\Vert_{\infty}+ \varepsilon\mu_j\log\left(\frac{2\max(n,m)}{\mu_j}\right)\right]}
\end{align*}
\end{lemma}
\begin{prv}
First remarks that  $\delta_0:=\Vert P^{(0)} - Q^{(0)}\Vert_1=0$.
Let $k\in\{1,...,I-1\}$ and let us denote $\delta_k:=\Vert P^{(k)} - Q^{(k)}\Vert_1$. Denote also in the following for all $k\in\{0,...,I-1\}$, $\widehat{C_1}^{(k)}:=-\varepsilon \log(\widehat{K_1}^{(k)})$. Therefore we have that
\begin{align*}
    \Vert P^{(k+1)} - Q^{(k+1)}\Vert_1\leq  \Vert P^{(k+1)} - \Pi(C(Q^{(k)})))\Vert_1 +
    \Vert \Pi(C(Q^{(k)})) - \Pi(\widehat{C_1}^{(k)})) \Vert_1 +  \Vert \Pi(\widehat{C_1}^{(k)})) -  Q^{(k+1)} \Vert_1
\end{align*}
Recall that $P^{(k+1)}=\Pi(C(P^{(k)})))$, therefore from Lemma~\ref{lem:error-cost}, we have first that:
\begin{align*}
     \Vert P^{(k+1)} - \Pi(C(Q^{(k)})))\Vert_1 \leq \frac{4\delta_k}{\varepsilon}\Vert D\Vert_{\text{op}}\Vert D'\Vert_{\text{op}}
\end{align*}
Moreover from Lemma~\ref{lem:error-approx-kernel}, we also have that 
\begin{align*}
     \Vert \Pi(C(Q^{(k)})) - \Pi(\widehat{C_1}^{(k)})) \Vert_1\leq \Vert \log(K_1^{(k)}/\widehat{K_1}^{(k)})\Vert_{\infty}
\end{align*}
Finally thanks Theorem 1 \todo{add prop in the main text at the end} in~\cite{dvurechensky2018computational}, we obtain that the Sinkhorn algorithm~\ref{alg-sink} outputs $u^{(k+1)},v^{(k+1)}$ such that $ Q^{(k+1)}:=\text{Diag}(u^{(k+1)}) \widehat{K_1}^{(k)}\text{Diag}(v^{(k+1)})$ satisfies $\Vert Q^{(k+1)}\mathbf{1}_n-a\Vert_1+ \Vert (Q^{(k+1)})^{T}\mathbf{1}_m-b\Vert_1\leq \mu_k$ in $\mathcal{O}\left(\mu_k^{-1}\log\left(\frac{1}{\iota \min_{i,j} \widehat{K_1}^{(k)}_{ij}}\right)\right)$ iterations where $\iota =\min\limits_{i,j}(a_i,b_j)$. Therefore thanks to Lemma~\ref{lem:error-sinkhorn}, we have finally that 
\begin{align*}
     \Vert \Pi(\widehat{C_1}^{(k)})) -  Q^{(k+1)} \Vert_1\leq  \mu_k + \sqrt{\frac{4}{\varepsilon}\left[ \mu_k (\Vert \widehat{C_1}^{(k)} \Vert_{\infty} + \varepsilon \mu_k \log\left(\frac{2\max(n,m)}{ \mu_k }\right) \right]}
\end{align*}
Therefore we obtain that
\begin{align*}
    \delta_{k+1}:=  \Vert P^{(k+1)} - Q^{(k+1)}\Vert_1\leq \alpha \delta_k + \beta_k
\end{align*}
from which the result follows by a simple induction.
\end{prv}
\begin{prop}
\label{prop:l1-error}
Let $I\geq 1$, $0<\delta\leq 1$ and $\tau\in(0,1)$. If for all $k\in\{0,..,I-1\}$
\begin{align}
%\label{eq:number-feature}
 r_k\in\Omega\left(\frac{\psi_k^2}{\mu_k^2}\log\left(\frac{n I}{\tau}\right)\right)
\end{align}
\begin{align*}
    \psi_{k}&:= 2^{d/2+1} \left(\frac{R_\ell^2}{4\varepsilon r W_0\left(R_\ell^2/\varepsilon r\right)}\right)^{d/2}\\
    R_k&:=\max\left(\Vert U^{(k)}\Vert,\Vert A\Vert\right)\\
    \mu_k&:=\frac{\varepsilon \delta_k^2}{200\left[R + 2 +  \log\left(\frac{2\max(n,m)}{\delta_k^2}\right)\right]}\\
    \delta_k&:=\min\left(\frac{\delta}{I},\frac{\delta}{I\alpha^{I-(k+1)}}\right)
\end{align*}
then we have with a probability of at least $1-\tau$ that:
\begin{align*}
    \Vert P^{(I)} - Q^{(I)}\Vert_1\leq \delta
\end{align*}
\end{prop}

\begin{prv}
First remarks that as soon as $r_k\in\Omega\left(\frac{\psi_{k}^2}{\mu_k^2}\log\left(\frac{n I}{\tau}\right)\right)$, thanks to Proposition 3.1\todo{add prop in the main text at the end} in ~\cite{scetbon2020linear} , we have with a probability of at least $1-\tau/I$
\begin{align*}
    \Vert\widehat{K_1}^{(k)}/K_1^{(k)}\Vert_{\infty}\leq 1 + \mu_k
\end{align*}
and that 
\begin{align*}
    \Vert \widehat{C_1}^{(k)}\Vert_{\infty}\leq \Vert C_1^{(k)}\Vert_{\infty} + \varepsilon \log(1 + \mu_k)
\end{align*}
Therefore we obtain that with a probability of $1-\tau/I$, 
\begin{align*}
   \beta_{k}\leq  \log(1 + \mu_k)+\mu_k +\sqrt{\frac{4}{\varepsilon}\left[\mu_k [\Vert C_1^{(k)}\Vert_{\infty} + \varepsilon\log(1 + \mu_k)]+ \varepsilon\mu_k\log\left(\frac{2\max(n,m)}{\mu_k}\right)\right]}
\end{align*}
Moreover remarks that for all $k\in\{0,,...,I-1\}$,
\begin{align*}
    \Vert C_1^{(k)}\Vert_{\infty}\leq \Vert C_1^{(k)}\Vert_{\text{op}} \leq R:=4 \Vert D\Vert_{\text{op}}\Vert D'\Vert_{\text{op}}
\end{align*}
and we obtain that 
\begin{align*}
     \beta_{k}\leq  2\mu_k +\sqrt{\frac{4}{\varepsilon} \mu_k [R +  \varepsilon\mu_k]}+ \sqrt{4\mu_k\log\left(\frac{2\max(n,m)}{\mu_k}\right)}
\end{align*}
Moreover as $\mu_k\leq 1$, we have that 
\begin{align*}
     \beta_{k}\leq  2\mu_k +\sqrt{\frac{4}{\varepsilon} \mu_k [R +  \varepsilon]}+ \sqrt{4\mu_k\log\left(\frac{8\max(n,m)}{\delta_k^2}\right)} + \sqrt{4\frac{\mu_k}{\delta_k^2}\log\left(\frac{\delta_k^2}{4\mu_k}\right)}\delta_k
\end{align*}
Finally by considering 
\begin{align*}
    \mu_k\leq \min\left(\frac{\delta_k}{12},\frac{\varepsilon \delta_k^2}{144[R +  \varepsilon]}, \frac{\delta_k^2}{144\log\left(\frac{2\max(n,m)}{\delta_k^2}\right)}, \frac{\delta_k^{2}}{200}\right) 
\end{align*}
we obtain that, 
\begin{align*}
     2\mu_k &\leq \frac{\delta_k}{6}\\
     \sqrt{\frac{4}{\varepsilon} \mu_k [R+1]}&\leq  \frac{\delta_k}{6}\\
     \sqrt{4\mu_k\log\left(\frac{2\max(n,m)}{\delta_k^2}\right)} &\leq \frac{\delta_k}{6}\\
     \sqrt{4\frac{\mu_k}{\delta_k^2}\log\left(\frac{\delta_k^2}{\mu_k}\right)}\delta_k &\leq \frac{\delta_k}{\sqrt{10}}\leq \frac{2\delta_k}{6}  
\end{align*}
Therefore we obtain that for such $\mu_k$
$$\beta_k\leq \delta_k.$$
Finally by an union bound and by applying Lemma~\ref{lem:total-error}, we obtain that 
\begin{align*}
        \Vert P^{(I)} - Q^{(I)}\Vert_1\leq \delta
\end{align*}
\end{prv}
We can now prove the theorem. Let $\delta>0$, $\tau\in(0,1)$. Thanks to Proposition~\ref{prop:l1-error}, as 
\begin{align}
\label{eq:number-feature}
 r_k\in\Omega\left(\frac{\psi^2}{\mu_k^2}\log\left(\frac{n I}{\tau}\right)\right)
\end{align}
where $\delta_k:=\min(\frac{\delta}{2L I},\frac{\delta}{2L K\alpha^{I-(k+1)}})$,
we have with a probability of at least $1-\tau$ that:
\begin{align*}
    \Vert P^{(I)} - Q^{(I)}\Vert_1\leq \frac{\delta}{2L}
\end{align*}
Finally applying Lemma~\ref{lem:GW-error} we obtain that 
\begin{align*}
     |\mathcal{E}_{D,D'}(P^{(I)}) - \mathcal{E}_{D,D'}(Q^{(I)})|&\leq \delta
\end{align*}
\end{proof}

\section{Useful Lemmas}

\begin{lemma}
\label{lem:error-cost}
Let $\delta>0$, $P_1,P_2\in\Pi(a,b)$ such that $\Vert P_1 - P_2 \Vert_1\leq \delta$, then
\begin{align*}
    \Vert \Pi(C(P_1)) - \Pi(C(P_2))\Vert_1 \leq \frac{4\delta}{\varepsilon}\Vert D\Vert_{\text{op}}\Vert D'\Vert_{\text{op}}
\end{align*}
\end{lemma}
\begin{prv}
From Proposition~2\todo{add prop in the main text at the end} in~\cite{altschuler2018massively}, we have that
\begin{align*}
    \Vert \Pi(C(P_1)) - \Pi(C(P_2))\Vert_1 &\leq \Vert \log(K(C(P_1))) -  \log(K(C(P_2)))\Vert_\infty\\
    &\leq\frac{1}{\varepsilon} \Vert C(P_1) -  C(P_2)\Vert_\infty\\
    &\leq \frac{1}{\varepsilon}\Vert C(P_1) -  C(P_2)\Vert_{\text{op}}\\
    & \leq \frac{14}{\varepsilon}\Vert P_1 - P_2\Vert_{1} \Vert D\Vert_{\text{op}}\Vert D'\Vert_{\text{op}}
\end{align*}
where we use the fact that $\Vert \cdot\Vert_\infty\leq\Vert \cdot\Vert_{\text{op}}\leq\Vert \cdot\Vert_1$ and that the operator norm is sub-multiplicative.
\end{prv}

\begin{lemma}
\label{lem:error-approx-kernel}
Let $\gamma>0$, $C_1, C_2\in\mathbb{R}^{n\times m}$ such that $\Vert K(C_1)/K(C_2)\Vert_{\infty}\leq 1 + \gamma$, then 
\begin{align*}
    \Vert \Pi(C_1) - \Pi(C_2)\Vert_1 \leq log(1 + \gamma)
\end{align*}
\end{lemma}
\begin{prv}
It follows directly from Proposition~2\todo{add prop in the main text at the end} in~\cite{altschuler2018massively}.
\end{prv}

\begin{lemma}
\label{lem:error-sinkhorn}
Let $C\in\mathbb{R}^{n\times n}$, $D_1$ and $D_2$ two positive diagonal matrices,  $P:=D_1K(C)D_2$ and let us denote $\delta:=\Vert P\mathbf{1}_n-a\Vert_1+ \Vert P^{T}\mathbf{1}_m-b\Vert_1$. Then if $\delta\leq 1$ we have
\begin{align*}
    \Vert P - \Pi(C)\Vert_1 \leq \delta + \sqrt{\frac{4}{\varepsilon}\left[\delta (\Vert C\Vert_{\infty} + \varepsilon\delta\log\left(\frac{2\max(n,m)}{\delta}\right) \right]}
\end{align*}
\end{lemma}
\begin{prv}
From Lemma~B\todo{add Lemma in the main text at the end} in~\cite{altschuler2018massively}, there exists $\widehat{P}\in\Pi(a,b)$ such that:
\begin{align*}
    \Vert P - \widehat{P}\Vert_1 \leq \delta 
\end{align*}
Therefore we have that:
\begin{align*}
    \Vert P - \Pi(C)\Vert_1 &\leq \Vert P - \widehat{P}\Vert_1 + \Vert \Pi(C) - \widehat{P}\Vert_1\\
    &\leq \delta + \Vert \Pi(C) - \widehat{P}\Vert_1
\end{align*}
Moreover, $f_C$ is $\varepsilon$-strongly convex with respect to the $\ell_1$-norm,
\begin{align*}
    f_C(\widehat{P}) \geq   f_C(\Pi(C)) +\langle \nabla f_C(\Pi(C)), \widehat{P} -\Pi(C) \rangle +\frac{\varepsilon}{2} \Vert \Pi(C) - \widehat{P}\Vert_1^2
\end{align*}
and as $\Pi(C)$ is the minimum of $f_C$ over $\Pi(a,b)$, we obtain that
\begin{align*}
    f_C(\widehat{P}) - f_C(\Pi(C)) \geq  \frac{\varepsilon}{2} \Vert \Pi(C) - \widehat{P}\Vert_1^2
\end{align*}
Moreover we have 
\begin{align*}
    |f_C(\widehat{P}) - f_C(\Pi(C))| \leq |f_C(\widehat{P}) - f_C(P))|  + |f_C(P) - f_C(\Pi(C))| 
\end{align*}
Moreover thanks to Lemma~B\todo{add prop in the main text at the end} in~\cite{altschuler2018massively} we have first that $\Vert \widehat{P} - P \Vert_1\leq \delta$, therefore we have by Lemma~E\todo{add prop in the main text at the end} in~\cite{altschuler2018massively}, 
\begin{align*}
    |f_C(\widehat{P}) - f_C(P))| \leq  \delta\Vert C\Vert_{\infty}+ \varepsilon\delta\log\left(\frac{2\max(n,m)}{\delta}\right)
\end{align*}
Moreover thanks to Proposition 3\todo{add prop in the main text at the end} in~\cite{altschuler2018massively}, we have also that:
\begin{align*}
    |f_C(P) - f_C(\Pi(C))| \leq  \delta\Vert C\Vert_{\infty}+ \varepsilon\delta\log\left(\frac{2\max(n,m)}{\delta}\right)
\end{align*}
Finally we obtain that 
\begin{align*}
     \Vert P - \Pi(C)\Vert_1 \leq \delta +\sqrt{\frac{4}{\varepsilon}\left[\delta\Vert C\Vert_{\infty}+ \varepsilon\delta\log\left(\frac{2\max(n,m)}{\delta}\right)\right]}
\end{align*}
\end{prv}

\begin{lemma}
\label{lem:GW-error}
Let $L:=\sup_{i,j,k,l}|D_{i,k}-D_{j,j}|^2$, let $P1,P2\in\Delta_{n\times m}$ and let us denote $\delta:=\Vert P1 - P2\Vert_1$. Then we have:
\begin{align*}
    |\mathcal{E}_{D,D'}(P1) - \mathcal{E}_{D,D'}(P2)|\leq 2L\delta
\end{align*}
\end{lemma}
\begin{prv}
We have
\begin{align*}
    |\mathcal{E}_{D,D'}(P1) - \mathcal{E}_{D,D'}(P2)|&\leq L \sum_{i,j,k,l} |P1_{i,j}P1_{k,l} - P2_{i,j}P2_{k,l}|\\
    &\leq L \sum_{i,j,k,l} |P1_{k,l} - P1_{k,l}|P1_{i,j} + |P1_{i,j} - P2_{i,j}|P2_{k,l}\\
    &\leq 2L\delta.
\end{align*}
\end{prv}
